# Supplementary material for: Bounds on oblivious multiparty quantum communication complexity
Source: arXiv:2210.15402 source file (2022-10-27)
Supplement: Supplementary file 1 [file Appendix.tex]

\appendix

\section{Relation between the communication models}\label{sec_app_relation}
With the oblivious routing condition, the ordinary communication model and the coordinator model have
the same communication complexity in asymptotic setting. To see why, let us prove
$\operatorname{QCC}_\Co(f, \varepsilon) \leq 2\operatorname{QCC}(f, \varepsilon)$
and $\operatorname{QCC}(f, \varepsilon) \leq \operatorname{QCC}_\Co(f, \varepsilon)$.
\begin{itemize}
\item $\operatorname{QCC}(f, \varepsilon) \leq \operatorname{QCC}_\Co(f, \varepsilon)$:
Suppose $\Pi \in \mathcal{P}_k(f, \varepsilon)_\Co$ is an optimal protocol.
Then, we can create another protocol $\tilde{\Pi} \in \mathcal{P}_k(f, \varepsilon)$ satisfying $\operatorname{QCC}(\tilde{\Pi}) \leq \mathrm{QCC}_\Co(\Pi)$
by  one player, say player 1, simulating the role of the coordinator in the protocol $\Pi$, in addition to the role of him/herself.
This means $\operatorname{QCC}(f, \varepsilon) \leq \operatorname{QCC}_\mathrm{Co}(f, \varepsilon)$.

\item $\operatorname{QCC}_\Co(f, \varepsilon) \leq 2\operatorname{QCC}(f, \varepsilon)$:
Suppose $\Pi \in \mathcal{P}_k(f, \varepsilon)$ is an optimal protocol.
Then, we can create another protocol $\tilde{\Pi} \in \mathcal{P}_k(f, \varepsilon)_\Co$ satisfying $\operatorname{QCC}_\Co(\tilde{\Pi}) \leq 2\mathrm{QCC}(\Pi)$
by the coordinator just passing messages, without performing anything, from player to player which is supposed to be sent in the protocol $\Pi$.
Note that each message is passed through player to coordinator and coordinator to player and therefore the factor of two appears in the inequality.
This means $\operatorname{QCC}_\Co(f, \varepsilon) \leq 2\operatorname{QCC}(f, \varepsilon)$.
\end{itemize}
The above proof also imply $\operatorname{QCC}^M_\Co(f, \varepsilon) \leq 2\operatorname{QCC}^M(f, \varepsilon)$
and $\operatorname{QCC}^{2M}(f, \varepsilon) \leq \operatorname{QCC}^M_\Co(f, \varepsilon)$.
\par
These explanations show that the power of these models are the same, up to the factor of two which is ignored, in asymptotic setting.
